# Supplementary material for: Deep Reinforcement Learning for Autonomous Cyber Defence: A Survey
Source: arXiv:2310.07745 source file (2024-09-27)
Supplement: Supplementary file 1 [file adoproof.tex]

\section{Theoretical Analysis of Approximate Double Oracles} \label{sec:adoproof}

Extending a proof from~\citep{oliehoek2018beyond} for GANs,
we can show that $\Exploitability \leq 0$ implies we 
have found an RBNE for ADO applied to MADRL: 
\begin{theoremsec}
If the termination condition from Equation  \ref{eq:termination_condition} is met, then an RBNE has been found.
\end{theoremsec}

\begin{proof}
It can be shown that $\Exploitability \leq 0$ 
implies that the agents have converged upon an RBNE:
\begin{equation}
\Exploitability = 
\G{i}{\JointPolicy{\O{i}{\pi^\mu_j})}{\pi^\mu_j}} +  
\G{j}{\JointPolicy{\pi^\mu_i}{\O{j}{\pi^\mu_i}}} \leq 0 = 
\G{i}{\JointPolicy{\pi^\mu_i}{\pi^\mu_j}} + 
\G{j}{\JointPolicy{\pi^\mu_i}{\pi^\mu_j}}
\end{equation}
Note that, as per Definition \ref{def:ABR},
\begin{equation} \label{eq:abr_property}
\G{i}{\JointPolicy{\O{i}{\pi^\mu_j}}{\pi^\mu_j}} \geq
\G{i}{\JointPolicy{\pi_i}{\pi^\mu_j}}
\end{equation}
for all computable $\pi_i \in \Pi^{O}_i$, where $\Pi^{O}_i$ is the set of ABRs that can be computed using an oracle $O$ for player~$i$. 
The same holds for player~$j$.
Therefore, the only way that Equation  \ref{eq:abr_property} could fail to hold, 
is if $\mu_i$ would include policies that are not 
computable (not in $\Pi_i^{O}$) that provide a higher payoff. 
However, the support of $\mu_i$ is composed of policies computed in previous iterations, therefore this cannot be the case. 
We conclude that 
\begin{equation}
\G{i}{\JointPolicy{\O{i}{\pi^\mu_j}}{\pi^\mu_j}} \geq 
\G{i}{\JointPolicy{\pi^\mu_i}{\pi^\mu_j}}
\end{equation}
for each agent.
Together with Equation \ref{eq:abr_property} this directly implies the following for each agent: 
\begin{equation}
\G{i}{\JointPolicy{\pi^\mu_i}{\pi^\mu_j}} = 
\G{i}{\JointPolicy{\O{i}{\pi^\mu_j}}{\pi^\mu_j}}. 
\end{equation}
We have therefore found an RBNE.
\end{proof}

%subsection{Linking Resource Bounded Nash Equilibrium with $\epsilon$-NE} \label{sec:RBNE_epsNE}
\begin{theoremsec}
Given sufficient resources to compute $\epsilon$-best responses, then an RBNE is an $\epsilon$-NE~\citep{oliehoek2018beyond}.
\end{theoremsec}

\begin{proof} \label{proof:RBNE_epsNE}
Starting from the RBNE with respect to the mixture profiles $\langle \mu_i, \mu_j \rangle$, we shall assume an arbitrary $i$.
By definition of an RBNE (Definition \ref{def:RBNE}): 

\begin{equation}
\G{i}{\JointPolicy{\pi^\mu_i}{\pi^\mu_j}}
\geq
\G{i}{\JointPolicy{\O{i}{\pi^\mu_j}}{\pi^\mu_j}}
\geq 
\max_{\mu'_i}
\G{i}{\JointPolicy{\pi^{\mu'_i}_i}{\pi^\mu_j}} - \epsilon.
\end{equation}
\end{proof}
