# Supplementary material for: Deep Reinforcement Learning for Autonomous Cyber Defence: A Survey
Source: arXiv:2310.07745 source file (2024-09-27)
Supplement: Supplementary file 2 [file envsoverview.tex]

\section{Environments Overview} \label{sec:envsoverview}

\subsection{Discretised Continuous Control Games}

%As a sub-function of Robotics, a field which has developed substantial interest in developing \RL
%in order to give autonomous functionality to machines, 
Continuous control is a well-furnished domain
containing many of the most complex, well-developed, and popular \envs.
%
%While many \envs exist in this category, %we have little interest in covering all of them,
%as 
Most continuous control \envs present similar challenges (in terms of those posed by \aco) to one another.
These challenges are summarised in~\autoref{tab:dcc}, under the column for 
MuJoCo~\citep{todorov2012mujoco,GymMuJoCoDocs}, a free and 
open-source physics engine which has been used to
develop many popular RL \envs for continuous control.
By design, these \envs are only intended to enable the training of control policies,
and as such are single-agent, neither stochastic nor partially observable, and not graph-based.
%
%It is worth noting that 
Stochasticity is present %in the \envs, but 
only in the starting positions of the body parts; 
the dynamics of %MuJoCo \envs 
are deterministic.

These \envs contain entirely continuous observations (usually joint angles,
positions, and velocities) and, by default, continuous actions too (torque applied to joints).
However, it is simple to quantize (\ie discretise) this action space and treat it as discrete.
One feature of note in these \envs is that there is potential for extensibility in
both the observation and action spaces.
{MuJoCo} \envs are similar in most ways, except for the goals and numbers of body parts.
By varying this number of body parts (as is possible by passing an argument to the {Swimmer}
\env, for example) one can create extensibility in both the observation and action spaces.
%
%In a novel addition, it may be possible to treat the body as a graph, by treating joints as nodes and
%body parts as edges connecting them.
%
%However, doing so would likely require significant development work, and while this would
%technically form a graph it is unlikely that it would lead to the presence of graph-based
%dynamics as in \aco.

While {MuJoCo} is of interest, other control \envs present challenges akin to \aco
far more clearly.
For example, the {Petting Zoo} \envs~\citep{PettingZooDocs} are extensions of the OpenAI Gym \envs
which are particularly designed for multi-agent training.
In this section, we look at the three Stanford Intelligent Systems Laboratory (SISL)
\envs~\citep{gupta2017cooperative,PettingZooDocs}, as these present a diverse and interesting range of challenges.
Some of these \envs ({Pursuit}, {Waterworld}) are adversarial in nature, and it may be possible to
extend the reward functions of others to be so.
In addition, these \envs confront agents with stochasticity and partial observability.
For example, in the {Multiwalker} \env, a number of bipedal robots attempt to carry
a package placed on top of them.
Each agent receives as its observations:
%\begin{itemize}
% \item 
accurate readings of its own physical properties;
%    \item 
LIDAR observations of the space in front and below itself;
%    \item 
Noisy information about neighbouring robots; and,
%    \item 
noisy observations of the object.
%\end{itemize}
%
This \env clearly contains stochasticity due to noise present in the agents' observations.
Additionally, partial observability is present, as the observations of each agent only contain
information about agents adjacent to itself.

The {Pursuit} \env is another SISL \env, where a number of pursuer agents must
move around a grid to avoid an obstacle and co-operatively capture adversary agents.
These adversaries move randomly, and the \RL-controlled pursuers have a limited sight range,
making this \env also stochastic and partially observable.
This \env, in fact, more closely represents a 2D game than a continuous control game,
but is included here for more relevant discussion.
Each agent in the \env has a multi-discrete observation space of size
$N \times N \times 3$ where $N$ is equal to the square observation range of each pursuer.
This also includes a potentially continuous dimension, as two of the three channels of this space
represent the number of pursuer and evader agents in each cell.
Given that the observation range and the size of the world space can be changed, this leads to a
potentially intractable observation space due to quadratic scaling.
Although the action space of the \env is simple (four movement directions and no-op),
the complex observation space makes this \env somewhat applicable to \aco.
However, while the rule-based and stochastic adversaries do improve the applicability of the
\env to \aco, the simplicity of the game means that even if \RL-based control
of the evaders could be implemented, it would not lead to particularly interesting behaviour, since
the evaders and pursuers both move at the same speeds.

\begin{table}[h]
\centering
\resizebox{\columnwidth}{!}{\includegraphics[width=\columnwidth]{envsummaries/dcc.pdf}}
\caption{An overview of domains that can be used 
for benchmarking discretized continuous control approaches 
and the extent to which they meet our criteria \wrt \aco \env properties.}
\label{tab:dcc}
\end{table}

The {Petting Zoo} \envs can be treated as single-agent \envs,
%the conversion of the \envs to single-agent \envs, 
by having a single model control all agents
within the \env.
While this would reduce or remove the level of partial observability in the \env as the combined
observable space of all agents would approach the whole state space, this would lead to vastly
increased observation and action space sizes as those of individual agents would be combined in to singular
spaces.
However, while this would increase the size of these spaces, it would not introduce any greater level
of scaling (\ie intractability) or new characteristics. 
Nevertheless, it is an option worth noting.

{Nocturne} ~\citep{nocturne2022} is a 2D driving simulator, built from the Waymo Open Dataset ~\citep{Sun_2020_CVPR}
in order to train agents to drive in a partially observable \env without having to handle direct sensor
inputs, \eg video from imaging cameras.
The \env %, which is multi-agent in nature, is neither zero-sum nor fully-cooperative; instead,
%it is mixed-motive
is a general-sum game, with each agent being required to both coordinate its own actions to reach its own goal
and cooperate with others to avoid conflict.
It is %heavily 
partially observable, with objects in the \env (both static and moving) causing occlusion
of objects behind (from the egocentric perspective of the agent).
However, it is not stochastic, with vehicle dynamics themselves being deterministic and simple.

The observation space of {Nocturne} is very large, consisting of the speeds, distances, and sizes of all
observed objects in the scene.
The \env caps the total number of observations at 6,727. 
However, it is noted that the actual number
of objects in a scene can exceed this, meaning the observation space could potentially be larger.
To make the \env more challenging, it may be feasible to re-frame the observation space as variable-length,
only including the objects which can currently be observed by the agent. 
This would form an interesting problem,
as the observation space would then become traditionally intractable.
However, the fact remains that the observation space would consist entirely of continuous values, limiting
the applicability of the challenge to \aco.
The action space, meanwhile, is a relatively small multi-discrete space, with continuous values for
acceleration, steering, and head tilting being split into discrete intervals.

It is feasible that the reward functions for the agents could be adjusted to form an adversarial
challenge, perhaps by punishing some agents for allowing others to complete their goals safely.
While this goes against the original intention of the \env (to provide a benchmark for safe driving)
the \env nevertheless makes this possible.

In summary, continuous control domain \envs offer significant challenges in terms of partial observability,
and multi-agent \envs in this domain could, with modification, possess some desirable properties,
such as adversarial training and large observation spaces.
However, the need to modify these \envs to do so is less than ideal, and certain desirable properties
such as being graph-based and traditionally intractable are generally missing, making this well-populated
area of \envs less than ideal for training agents to tackle the challenges posed by \aco.

\subsection{Gridworld Domains and 2D Games}

\begin{table}[h]
\centering
\resizebox{\columnwidth}{!}{\includegraphics[width=\columnwidth]{envsummaries/gd2d.pdf}}
\caption{Here, we provide an overview of Gridworld and 2D Game environments, including 
Categorised N-Rooms (CNR), Selective Predator-Prey (SPP), Multi-Step Plan Environment (MSPE), 
Platform Jumping (PJ), MicroRTS (MRTS), Pommerman (PM), DinerDash (DD), and Half Field Offense (HFO).
Again, we evaluate the extent to which each environment meets our desirable properties.}
\label{tab:gd2d}
\end{table}

Gridworld domains are relatively simple \envs where, generally, an agent must navigate a grid by moving
in one of four cardinal directions at each timestep while observing obstacles, goals, or other agents in
surrounding squares.
2D games are often similarly simple, but more varied, and may include more complex dynamics such as physics,
continuous observations or actions, or sensor-based observations.
The previously-discussed {Pursuit} and {Multiwalker} games are examples of the gridworld and 2D game domains,
respectively.
However, these \envs have far more to offer in terms of challenges relevant to \aco, and indeed,~\autoref{tab:gd2d}
is well-populated.

One advantage of gridworld and 2D games is that they are very simple to create and modify.
{Categorised N-Rooms}~\citep{zahavy2019learn} is an example of this.
This is a gridworld game where the states of each square are randomly assigned to one of $k$ categories.
The agent is tasked with moving to a goal position, but has a greater chance to move if it takes an action
corresponding to the category of the square it intends to move to.
This results in a multi-discrete action space which can be extended simply by changing the value of $k$.
For example, with $k = 1,000$, there are 1,000 actions for each cardinal direction, leading to an action
space size of 4,000.
The observation space in this case would be similarly large.
For a grid of shape $N \times N$, the multi-discrete observation space of the agent would be
$N \times N \times k$.
With both $N$ and $k$ being easily changed, this can lead to observation spaces
which become intractably large.
Furthermore, the \env itself is stochastic, as movement is probabilistic.
Should an agent correctly select an action with a category corresponding to the square it intends to move to,
the probability of moving to it is $0.75$; if the category chosen is incorrect, the agent may still move,
with a probability of $0.5$.
While this \env is simplistic, as expanding the observation and action spaces does not introduce any greater
complexities in dynamics, it demonstrates that this \env can provide challenges applicable to \aco in
a simple \env which could feasibly be implemented with little effort.

{Selective Predator-Prey} ~\citep{song2019solving,PredatorPreyExample} is an adversarial 2D game which is
similar in nature to {Pursuit}, in that multiple predators are tasked with chasing and catching multiple prey.
In this game, however, a single agent controls the predators by design, observing the positions of all agents
(predator and prey) and assigning commands to $k$ predators.
The agent is rewarded when two or more predators catch a prey.
While not available in code, it would be a simple task to 
enable adversarial learning, 
%extend this \env to an adversarial learning scenario,
by having a second agent control the prey.
Since this \env, unlike {Pursuit}, is fully observable, the observation space instead consists of the
positions of every agent in the game.
In this way, the observation space size can be controlled by varying the number of agents in the game, causing
extensibility.
%%
%Further, another simple modification would be to vary the observation size, with it reducing as the number
%of prey agents left in the game reduces.
%%
%While not representative of the \aco problem, this would lead to an interesting challenge whereby the
%game becomes less complex as learning progresses.
%%
%In a similar manner to the observation space, the action space grows with the number of predator (or prey,
%in the multi-agent scenario) agents.

Within the {Multi-Step Plan Environment}~\citep{dulac2015deep} %is a gridworld \env where 
a single agent must
navigate towards a goal with a limited visibility range.
The \env sets the goal location to always be at the bottom-right of a gridworld, with the agent
being limited to moving down and right. 
The novelty in this \env lies in the action space -- rather than choosing a single movement action per
timestep, the agent must choose its next $N$ actions.
Reaching the goal, while not guaranteed, is trivial.
The challenge is for the agent to reach its goal in as few steps as possible.
Given that at each timestep, the agent can only choose one of two actions, the action space size becomes
$2N$.
While this is extensible, and technically may become intractable as the planning horizon grows, it is
nevertheless rather simplistic.
A multi-step planning \env with a greater choice of actions at each timestep would, however,
pose a greater challenge.
\reportonly{
Grouped actions such as this are investigated further in~\cite{PBS123CARLReport}.
}

{MicroRTS}~\citep{huang2021gym} is a simple Real-Time Strategy (RTS) game. %which 
It is designed to enable the training of \RL agents on an \env which is similar to {PySC2}~\citep{vinyals2017starcraft}; the \RL
\env adaptation of the popular RTS game \sctwo which possesses huge complexity. 
Therefore, MicroRTS is a lightweight version of PySC2, without the extensive
(and expensive) computational requirements.
The game features a gridworld-like observation space, where for a map of size $h \times w$, the observation space
is of size $h \times w \times f$, where $f$ is a number of discrete features which may exist in any square.
This observation space can be set to be partially observable.
The action space, however, is a much larger multi-discrete space, where each worker is commanded with a total
of seven discrete actions.
The number of workers will change during the game, however, making the core RTS action space intractable.
In order to handle this, the authors of {MicroRTS} implemented action decomposition as part of the \env,
and the action space is separated in to the unit action space (of 7 discrete actions), and the player action
space.
While the authors discuss two formulations of this player action space, the one which is documented in code is
the {Gridnet} approach, whereby the agent predicts an action for each cell in the grid, with only the
actions on cells containing player-owned units being carried out.
This leads to a total action space size of $h \times w \times 7$, which could potentially be extremely large.
The challenge of varying numbers of agents is remarkably similar to the challenge of varying numbers of
nodes in \aco, and the {MicroRTS} \env, if action decomposition were to be stripped away, would be a
strong candidate for handling large and variably-sized discrete action spaces.

{Pommerman} ~\citep{DBLP:journals/corr/abs-1809-07124} is an open-source clone of the classic 2D game
{Bomberman}, involving a 4-player adversarial game on a $N \times N$ gridworld (configurable).
The action space of this \env is simple, consisting of a few actions similar to other gridworlds, but
the observation space is large, consisting of multiple discrete values per grid cell, as well as several
extraneous discrete and continuous values.
Furthermore, it is possible to configure the game as a 2v2 team game, where the observation space becomes
partially observable, and teammates must communicate (using a dedicated discrete value present in both the
observation and action spaces) in order to gain information from outside their field of view.
However, while this large observation space and mixed cooperative-adversarial game does present some unique
and interesting challenges, these alone do not align well to the \aco problem due to dissimilar game dynamics
and a lack of extensible or intractable observation or action spaces.

\subsection{Network-Based Environments}

\begin{table}[h]
\centering
%\resizebox{\columnwidth}{!}{\includegraphics[width=\columnwidth]{\maketable}}
\resizebox{\columnwidth}{!}{\includegraphics[width=\columnwidth]{envsummaries/nbd.pdf}}
\caption{An overview of network-based \envs, including: Intelligent Communication Jamming (ICJ), 
Multicast Scheduling Problem (MSP) , Gym-ANM, SUMO, Iroko}
\label{tab:nbd}
\end{table}

Networks are an integral component of many domains.
Computer networks and power grids are both intuitive examples of this, as physical wires connecting hardware in
graph-like structures are present.
However, other domains incorporate networks too. 
For example, road networks, where roads connect intersections.
These domains are of particular interest as \aco, too, is a network-based domain.
And by the nature of network-based domains, they contain graph structures, which are scarce in most other domains.
This section analyses \RL \envs from such domains, summarised in \autoref{tab:nbd}.

{Intelligent Communication Jamming} ~\citep{e24101441} is a scenario whereby an agent must learn to jam the
communications of others by selecting the correct modulation mode, transmission power and frequency.
Each of these makes up a dimension of the action space, and does so twofold in the observation space (as the parameters
of both the agent and its adversary are present) -- leading to both being large, discrete spaces.
The size of these dimensions (which could conceivably be extended beyond what is specified in the paper)
combinatorially form spaces which are traditionally intractable due to their size.
Further, the potentially adversarial nature of the game, as well as its stochasticity, make it a simple but attractive
option for testing methods for tackling large observation and action spaces.

{Gym-ANM} ~\citep{HENRY20211000921,HENRY20211000922} is a framework for designing \RL \envs that model
Active Network Management tasks in electricity distribution networks.
The criteria logged in ~\autoref{tab:nbd} for this \env are properties of the {ANM6-Easy} \env
which is provided with the code base.
However, as denoted, the framework makes it easy to write extensions to allow for greater challenges.
Of note is that the \env contains graph-based dynamics, as it is based around a power grid, and could be
extended to include stochasticity and partial observability.
However, the continuous (although extensible) observation and action spaces limit this \env's applicability
to \aco problems.

{SUMO}~\citep{SUMO2018} is a traffic simulation tool which allows for the implementation of complex, distributed
traffic light control scenarios.
While neither Python-based nor intended for \RL, there exists a third-party interface for fulfilling
these criteria ~\citep{sumorl}.
There are two configurations for this \env; single-agent, and multi-agent.
For this review, we consider the multi-agent configuration, but treat it as a single-agent problem, since
while the multi-agent scenario introduces greater complexity with multiple junctions needing to be controlled, it does
not necessitate the use of multiple agents.
The goal of an agent in {SUMO} is to control traffic signals at junctions in order to minimise the delay of
vehicles passing through.
The observation space is a small, but extensible (\wrt the number of junctions) %(as the simulation can be extended to any number of junctions)
continuous space, containing information about the amount of traffic in incoming lanes.
The action space, however, is more novel.
Each set of lights is controlled by a single discrete variable, each of which corresponds to a configuration of lights
which results in a different flow of traffic.
For example, at a two-way single intersection, there are 4 possible configurations.
Each intersection type has a different number of configurations, however, meaning that the action space is not
only multi-discrete, but also uneven.
Further, as the intersections are connected by roads in the simulation, the \env will inevitably
contain graph-like dynamics, \ie the actions at -- and traffic through -- each intersection will affect the state at
connected junctions.
As such, the action space and \env dynamics of {SUMO} are applicable to \aco.
However, the small observation space and lack of adversarial or partially observable properties
limit this applicability.

Network-based \envs often contain graph-based dynamics.
Given this, and the fact that \aco is itself a network-based domain, one would expect the \envs presented
here to translate well to \aco.
However, the presence of continuous observation and action spaces, as well as a general lack of complex properties
such as partial observability and adversarial scenarios, make these \envs less suitable for testing approaches
to \aco than one would hope.
However, \envs such as {SUMO} which do have some of these properties, and frameworks such as {Gym-ANM} which
enable one to create them, may present some opportunities for development in this area.

\subsection{Recommender Systems}

\begin{table}[h]
\centering
\resizebox{\columnwidth}{!}{\includegraphics[width=\columnwidth]{envsummaries/rs.pdf}}
\caption{An overview of recommender system gym \envs, including: 
User Simulation Environment (USE), RecoGym, RecSim, RL4RS.}
\label{tab:rs}
\end{table}

The domain of Recommender Systems is one which a variety of approaches are applicable to, not only \RL.
However, despite traditionally being a domain where datasets are used to derive solutions with supervised learning,
\RL has recently become a technology of interest in the domain, and as such, several \RL \envs for training
agents to perform recommendation tasks have emerged.
The recommender systems task is a challenging one for a number of reasons, but in particular, the large (often well in
excess of 100,000) number of potential products to choose recommendations from makes the task challenging for
all ML approaches.
In the case of \RL approaches, this translates to intractably large observation and action spaces, so much so
that the {Slate-MDP} problem formulation has been developed in order to tackle the challenge~\citep{sunehag2015deep}.
Nevertheless, the potential for large, discrete observation and action spaces makes this domain one worth searching
for \envs which pose challenges similar to \aco, as summarised in \autoref{tab:rs}.

The {User Simulation Environment} ~\citep{ie2019reinforcement} is a stylised recommender \env
designed to enable experimentation with {Slate-MDPs}.
Because of this, the large number of products are aggregated and simplified into slates for the action space;
however, if one were to implement this \env (which is thoroughly described) in code, choosing not to
implement this slate aggregation would expose a multi-discrete (as multiple products are recommended at once) action
space which could potentially be extended to the point of intractability.
The \env described also contains a mixed discrete-continuous observation space, partial observability,
and potentially stochasticity. 
As such, this simple \env design could be suitable for developing
approaches to large action spaces which are applicable to \aco.

{RecSim}~\citep{ie2019recsim} is a configurable framework for creating RL \envs for recommender systems.
In {RecSim}, an agent observes multiple sets of features from both a user and a document database, and makes document
recommendations based on these.
These sets of features are comprised of features from the user, their responses to previous recommendations, and
the available documents for recommendation.
These observations fulfil all desirable criteria related to observation spaces. 
Not only are they stochastic (due to
randomness in the user's behaviour) and partially observable (due to incompleteness in the visible user features),
but they are also an extensible mix of discrete and continuous features which scale exponentially with both the
number of documents and the number of features extracted from them.
As such, the observation space of {RecSim} poses a significantly complex challenge similar to that presented in \aco.
The action space, however, is less remarkable.
The agent must choose a number of documents to recommend, which is a multi-discrete space which is potentially
extensible as the number of recommendations and documents increases.
However, this is unlikely to be intractable unless the number of documents becomes vast.
Nevertheless, this large space complements the novel and complex observation space, making this a strong candidate
for experimenting with approaches for \aco challenges.

\subsection{Miscellaneous Games}

\begin{table}[h]
\centering
\resizebox{\columnwidth}{!}{\includegraphics[width=\columnwidth]{envsummaries/mg.pdf}}
\caption{An overview of games that do not fit into any of the other categories, including 
the text-based game Zork, the card game Dou Dizhu, and the \sctwo based SMAC.}
\label{tab:mg}
\end{table}

This section covers miscellaneous \envs which do not fit in to any other category (See~\autoref{tab:mg}).
As such, they cannot be compared to one another based on their domain, and should be treated independently.

Zork~\citep{zahavy2019learn} is a text-based game where the agent must interact via a text interface. 
In each state the agent has to choose from over a thousand possible actions. 
License prohibits commercial use of the environment. 

{Dou Dizhu} ~\citep{pmlr-v139-zha21a} is a three-player card game where two players must team up against
a joint adversary called a {landlord} in order to win.
%
%When implemented as an \RL \env, this game forms a 
It is a complex, multi-agent, and adversarial game.
The multi-discrete observations of cards in the agent's hand and others' is partially observable,
as opponents' cards are not all visible.
In addition, the action space is a large multi-discrete space which is traditionally
intractable.
This is due to the agent needing to choose a valid combination of cards, with valid combinations being of variable
length.
In addition to being adversarial, the game also involves cooperative gameplay between the two players not selected
as {landlord}.
This \env could potentially offer a simple route for developing approaches to \aco problems, and
while the dynamics of the \env are not similar, the properties are relevant.

{SMAC}~\citep{samvelyan19smac,ellis2022smacv2} is a benchmarking \env for research in the field of
collaborative MARL, and makes use of the \sctwo game mentioned previously.
In the centralised version of this game, the player controls multiple in-game agents, the number of which can
vary throughout an episode.
The player receives observations from each agent's surroundings, forming an observation space which fulfils most
desirable criteria, containing mixed multi-discrete and continuous types, extensibility and intractability, and
partial observability.
Similarly, the multi-discrete action space consists of a set of actions which can be taken for each agent, which is
therefore also extensible and intractable.
All of these factors, combined with the stochasticity of the \env, make {SMAC} (and \sctwo in general)
an excellent \env for developing approaches to tackling challenges in \aco.
However, this complexity is also a drawback, as the game is notorious for requiring large amounts of computation
to learn well, hence the development of smaller and simpler \envs such as {Micro-RTS}.
