# Supplementary material for: Deep Reinforcement Learning for Autonomous Cyber Defence: A Survey
Source: arXiv:2310.07745 source file (2024-09-27)
Supplement: Supplementary file 3 [file sota_drl_approaches.tex]

\section{Deep Reinforcement Learning} \label{sota_drl_approaches}

\subsection{Deep Q-Learning} \label{sec:rl:dqn}

In DRL multi-layer Deep Neural Networks (DNNs) are used
to approximate value functions or, as we shall see below, 
even learn a parameterized policy. 
%
%Various types of DNN architectures have been utilized by DRL agents, including
%fully connected, convolutional to process image observations, and graph neural
%networks to facilitate the training of agents within domains that can be 
%modelled using a graph -- such as \target. 
%
%We shall discuss different types of DNNs in 
%\autoref{sec:function_approximators}. 
%
We shall assume a DNN with parameters
$\theta$ and sufficient representational capacity 
to learn our required 
approximations. 
For Deep Q-learning (DQN), DNNs map a set of $n$-dimensional state 
variables to a set of $m$-dimensional Q-values 
$f:\rats^n \to \rats^m$~\citep{mnih2013playing,mnih2015human}. 
Here, $m$ represents the number of actions available to the 
agent. 
The parameters~$\theta$ are optimized via stochastic gradient descent, 
by randomly sampling past transitions 
%state transition tuples $\left(\state,\action,\state',r\right)$
%that are 
stored within an experience replay memory $\mathcal{D}$ 
\citep{lin1992self,mnih2015human,schaul2015prioritized,mousavi2016deep}. 
The DNN is trained to minimize the time dependent loss function,
\begin{equation}\label{eq:time_dependent_loss_function}
L_k\left(\theta_k\right) = \mathbb{E}_{(\state,\action,\state',r) \sim U(\mathcal{D})}\Big[ \left(Y_k - Q\left(\state,\action; \theta_k\right)\right)^2 \Big],
\end{equation}
where $(\state,\action,\state',r) \sim U(\mathcal{D})$ represents mini-batches of experiences drawn uniformly at random from 
%the set of samples stored 
%inside 
$\mathcal{D}$, $t$ the current iteration, and $Y_k$ is the target:
\begin{equation} \label{eq:DQNTarget}
Y_k \equiv r + \gamma Q(\nextstate, \argmax_{\action \in \mathcal{U}} Q(\nextstate, \action; \theta_k);\theta_{k}').
\end{equation}

Equation \eqref{eq:DQNTarget} uses Double Deep Q-learning (DDQN) \citep{hasselt2010double}, 
where the target action is selected using weights 
$\theta$, while the target value is computed using weights $\theta'$ from a target network. 
%
%The target network is a more stable version of 
%the current network. 
Using the current network rather than the target network for the target value estimation 
decouples action selection and evaluation for more stable updates.
Weights are copied from the current to the target network after every $n$ transitions~\citep{van2016deep}
or via a soft target update 
%using a rolling convex combination
~\citep{lillicrap2015continuous}. 
DDQNs have been shown to reduce overoptimistic value estimates~\citep{van2016deep}.
