# Supplementary material for: Deep Reinforcement Learning for Autonomous Cyber Defence: A Survey
Source: arXiv:2310.07745 source file (2024-09-27)
Supplement: Supplementary file 4 [file additional_envs.tex]

\subsection{Extensive summary of environments} \label{appendix:env_summary}

Below we provide a summary of the evaluation domains that we encountered
while conducting our literature review. 
The majority of the domains did not meet all three of our criteria
with respect to confronting learners with the same challenges 
as \aco, namely: high-dimensional action and state spaces,
as well as being adversarial.
Nevertheless, the domains are useful for evaluating approaches
for these problems individually (or sometimes more). 
We also argue that: i.) there is a need in this area of 
the literature for a benchmarking suit with a standard
set of challenges that approaches can be benchmarked on,
and ii.) even single agent domains can be converted
into adversarial domains through the addition of 
an adversarial \say{nature} agent, giving rise
to \emph{robust adversarial reinforcement learning}\cite{pinto2017robust}.
This can be in the form of domain modifications, or simply through 
the adversary perturbing the protagonist agent's actions.

\subsubsection{Gridworlds} \label{app:envs:sub:gridwolrds}

\begin{table}[h]
\resizebox{\columnwidth}{!}{
\begin{tabular}{ |p{3cm}||p{6cm}|p{1.5cm}|p{1.5cm}|p{1cm}|p{1cm}|}
 \hline
 \multicolumn{6}{|c|}{\textbf{Environments Overview}} \\
 \hline
 \textbf{Name} & % Name of the aglo
 \textbf{Description} &  % Wolpertinger | Action Decomposition | Action Elimination | Hierarchical 
 \textbf{HD-$\states$}  &  % Brief summary of the approach
 \textbf{HD-$\actions$}  &  % MDPs, POMDPs, Slate-MDPs, Dec-POMDPs, etc
 \textbf{Adv.} &  % MDPs, POMDPs, Slate-MDPs, Dec-POMDPs, etc
 \textbf{Code} \\  % MDPs, POMDPs, Slate-MDPs, Dec-POMDPs, etc
\hline
\hline
\multicolumn{6}{|c|}{\textbf{Gridworld Domains / 2D Games}} \\
\hline
Categorised $N$-Rooms~\cite{zahavy2018learn} & Gridworld domain where states are randomly assigned to $k$ categories. The agent is tasked with reaching a goal position, but can only move if it takes an action with the correct category. There are therefore $4k$ actions. The move is random with a probability 0.75 if the category is correct, otherwise 0.5. & \xmark & \checkmark & \xmark &  \xmark \\
\hline
\textbf{Selective Predator-Prey}~\cite{song2019solving} & Multiple predators are tasked with capture randomly moving preys (although for adversarial learning one could imagine learning prey). The agent observes the position of all agents (predators and prey), selects $K$ predators, and assigns commands. A reward is given when two predators catch a prey. & \boldcheckmark & \boldcheckmark & \boldcheckmark & \boldcheckmark~\tablefootnote{\url{https://github.com/DeUmbraTX/practical_rllib_tutorial/blob/main/your_rllib_environment.py}} \\
\hline
Multi-Step Plan Environment~\cite{dulac2015deep} &  Construct an $n$-step plan using all possible actions across $n$ steps, \ie the agent has $i$ actions available at each time step and an agent needs to plan $n$ time steps into the future. & \xmark & \checkmark & \xmark & \xmark \\
\hline
Platform Jumping~\cite{wei2018hierarchical} & Simple 2d game in which an agent must move and jump across platforms while avoiding enemies. & \xmark & \checkmark & \xmark & \xmark \\
\hline
\hline
\end{tabular}}
\caption{An overview of evaluation environments and their properties with respect to the 
defined suitable environment criteria. In this table the columns HD-$\states$ and HD-$\actions$ 
refer to state and action spaces that are intractable for traditional reinforcement 
learning approaches, while Adv. denotes adversarial environments.}
\label{tab:environments:gridworlds}
\end{table}

Gridworld domains are frequently observed within the reinforcement learning literature
as means to conduct preliminary evaluations to verify that an approach has some merit.
They provide a low-threshold means through which to construct scenarios 
that have relevant properties comparable to an intended target domain. 
Due to their popularity, there are numerous repositories available online that allow
one to specify gridworld scenarios with ease~\footnote{\url{https://github.com/bjkomer/gym-maze}}. 
Gridworlds have also provided a means through which to construct evaluation scenarios 
for approaches designed to address the high-dimensional action space problem. 

\textbf{Selective predator-prey:} 
Song et al.~\cite{song2019solving} propose a selective predator-prey
scenario that involves multiple predators that have to capture randomly moving 
preys that are distributed throughout the environment.
The environment is fully observable from the perspective of the agent, who must
at east time step select $K$ predators and assign each a command (the direction
to move in). 
Only the selected predators move according to the selected actions, and capture 
the prey.
In addition, two predators must pounce on the prey in order for a reward to be obtained.
The domain is interesting in that it features a high-dimensional combinatorial action space,
and also, depending on the domain configuration, potential challenges with respect to 
the dimensionality of the observation space.
In a  sufficiently sized grid, feeding the agents the complete observation space will 
likely not be feasible, and therefore other representations would need considering 
(\eg graph based, or partial observations). 
Finally, Song et al.~\cite{song2019solving} had randomly moving prey, in principle their
movements could also determined by a learning agent (or multiple-learning agents), adding
an adversarial dimension to this game. 

\textbf{Categorised $N$-Rooms:}
In this domain, introduced by Zahavy~\cite{zahavy2018learn}, the 
agent is situated within a gridworld with $N$ rooms. 
The agent is tasked with reaching a goal cell, receiving a penalty 
after each step, and a reward of 0 upon reaching the goal.
The agent can move in four directions (up, down, left, right).  
However, the task is complicated by the fact that each state of the
game is randomly devided into $K$ categories at the start. 
At each step the agent must choose among $4 \times K$ actions.
The agent will move in the intended direction with a probability
of 0.75 if the correct category is selected.
Otherwise the probability is 0.5.

\textbf{Platform Jumping:} 
Confronts learners with a Parameterized-Action MDP, 
where an agent must jump across platforms while 
avoiding avoiding enemies~\cite{wei2018hierarchical}.
Discrete actions in this domain represent run, jump (over
enemies) and leap (across platforms), 
while the continuous action is speed.  

\textbf{Multi-Step Planning:} 
The multi-step planning problem confronts the agent with the challenge of having to 
construct an $n$-step plan using all possible actions across the next $n$ steps~\cite{dulac2015deep}.
As result, if the agent can choose among $i$ actions, and needs to plan $n$ steps
into the future, there are $i^n$ possible actions.
The authors implement problem setting on a puddle world environment, 
where each cell can have four types: empty, puddle, start, or goal. 
A reward of $-1$ is obtained for visiting an empty cell, $-3$ for visiting 
a puddle, and $250$ upon reaching the goal. 

\subsubsection{Domains with graph-based states}

\begin{table}[h]
\resizebox{\columnwidth}{!}{
\begin{tabular}{ |p{3cm}||p{6cm}|p{1.5cm}|p{1.5cm}|p{1cm}|p{1cm}|}
 \hline
 \multicolumn{6}{|c|}{\textbf{Environments Overview}} \\
 \hline
 \textbf{Name} & % Name of the aglo
 \textbf{Description} &  % Wolpertinger | Action Decomposition | Action Elimination | Hierarchical 
 \textbf{HD-$\states$}  &  % Brief summary of the approach
 \textbf{HD-$\actions$}  &  % MDPs, POMDPs, Slate-MDPs, Dec-POMDPs, etc
 \textbf{Adv.} &  % MDPs, POMDPs, Slate-MDPs, Dec-POMDPs, etc
 \textbf{Code} \\  % MDPs, POMDPs, Slate-MDPs, Dec-POMDPs, etc
\hline
\hline
\multicolumn{6}{|c|}{\textbf{Domains with graph-based States}} \\
\hline
DinerDash~\cite{chen2020dinerdash} & A waitress agent is tasked with running a restaurant via a large combinatorial action space. & \xmark & \checkmark & \xmark & \checkmark~\tablefootnote{\url{https://github.com/AdaCompNUS/diner-dash-simulator}} \\
\hline
\end{tabular}}
\end{table}

\textbf{DinerDash}:
Chen et al.~\cite{chen2020dinerdash}
introduce a gym environment where the agent is 
tasked with running a restaurant through controlling a waitress.
The objective is to serve as many customers as possible. 
The domain configuration illustrated in \cite{chen2020dinerdash} 
has the waitress serving six tables of different sizes and up to 
seven waiting groups. 
The size of the groups can vary.
The agents actions consist of: 
allocating each group to a table; 
collecting orders; 
submitting orders;
picking up food;
collecting bills;
cleaning the tables;
and returning dishes to the dish collection point.
Rewards are determined by a happiness value for each group
of customers.
The happiness value will decrease if the customers wait for too long, 
and once the happiness value reaches zero, the customer will leave.
This results in the player losing a life -- each episode starts with the
player having five lives.
The configuration depicted in \cite{chen2020dinerdash} has a 40 
dimensional state space, and 57 actions.
Although given the problem definition, scaling up the scenario
to a larger state and action space is feasible, \eg, through 
increasing the number of tables, adding addition.

\subsubsection{Discretised Continuous Control Domains} \label{Sec:DCCD}

\begin{table}[h]
\resizebox{\columnwidth}{!}{
\begin{tabular}{ |p{3cm}||p{6cm}|p{1.5cm}|p{1.5cm}|p{1cm}|p{1cm}|}
 \hline
 \multicolumn{6}{|c|}{\textbf{Environments Overview}} \\
 \hline
 \textbf{Name} & % Name of the aglo
 \textbf{Description} &  % Wolpertinger | Action Decomposition | Action Elimination | Hierarchical 
 \textbf{HD-$\states$}  &  % Brief summary of the approach
 \textbf{HD-$\actions$}  &  % MDPs, POMDPs, Slate-MDPs, Dec-POMDPs, etc
 \textbf{Adv.} &  % MDPs, POMDPs, Slate-MDPs, Dec-POMDPs, etc
 \textbf{Code} \\  % MDPs, POMDPs, Slate-MDPs, Dec-POMDPs, etc
\hline
\multicolumn{6}{|c|}{\textbf{Discretised Continuous Control Domains}} \\
\hline
\textbf{Discretised Continuous Control Domains}~\cite{tavakoli2018action,gupta2017cooperative,metz2017discrete} & Typically discretised MuJoCo domains. Domains could in principle be made adversarial by incorporating ideas from the robust adversarial reinforcement learning literature~\cite{pinto2017robust,zhang2020stability,dennis2020emergent}~\footnote{Arguably robust adversarial reinforcement learning (RARL) could be applied to most of the domains here. However, RARL is particularly relevant for continuous control domains, where it has a strong track record of improving the robustness of agents.}. Can in principle also include high-dimensional observation spaces.  & \boldcheckmark & \boldcheckmark & \boldcheckmark & \boldcheckmark~\tablefootnote{MuJoCo continuous control domains are available within the Open AI Gym (\url{https://github.com/openai/gym}). Cooperative multi-agent continuous control domains are available via the PettingZoo (\url{https://pettingzoo.farama.org/environments/sisl/})}  \\
\hline
\hline
\end{tabular}}
\end{table}

Discretised continuous control domains (\eg., environments
are simulated using the MuJoCo physics engine~\cite{todorov2012mujoco})
have become a popular means through which to obtain
high-dimensional MultiDiscrete action spaces for 
evaluating proposed approaches~\cite{dulac2015deep,tavakoli2018action}.
Within these domains each action dimension $d = \{1, ...,N\}$ of the original continuous
control action space is discretized into $i$ segments, resulting
in an action space with $\rvert\actions\rvert = i^d$ actions~\cite{dulac2015deep,tavakoli2018action}.
Depending on the granularity of the discretization, one can 
construct intractable action spaces with ease within these domains,
as demonstrated in \autoref{tab:disc_cont_envs}, listing the
number of combinatorial actions with a discretization of $n=33$
actions for each actuator. 
\begin{table}
\resizebox{\columnwidth}{!}{
\begin{tabular}{ |p{2.5cm}||p{7cm}|p{4cm}|p{5cm}|} %p{3cm}|   }
 %\hline
 %\multicolumn{4}{|c|}{Discretized Continuous Environments - Domain Properties} \\
 \hline
 \textbf{Domain} & \textbf{Observation Space Dimension dim($o$)} & \textbf{Action Dimensions $N$} & \textbf{$n^N$ combinatoral actions} \\ %& BDQ Network Outputs ($n \times N$) \\
 \hline
 Reacher-v1    & 11  & 2 & $1.1 \times 10^3$ \\% & 66\\
 Hopper-v1     & 11  & 3 & $3.6 \times 10^4$ \\% & 99\\
 Walker2d-v1   & 17  & 6 & $1.3 \times 10^9$ \\% & 198\\
 Humanoid-v1   & 376 & 17 & $6.5 \times 10^{25}$ \\% & 561\\
 \hline
\end{tabular}}
\caption{Dimensionality and number of actions using a granularity of $n=33$, a setting 
used by \cite{tavakoli2018action}.}
\label{tab:disc_cont_envs}
\end{table}

\subsubsection{Text Based Games} \label{sec:text_based_games}

\begin{table}[h]
\resizebox{\columnwidth}{!}{
\begin{tabular}{ |p{3cm}||p{6cm}|p{1.5cm}|p{1.5cm}|p{1cm}|p{1cm}|}
 \hline
 \multicolumn{6}{|c|}{\textbf{Environments Overview}} \\
 \hline
 \textbf{Name} & % Name of the aglo
 \textbf{Description} &  % Wolpertinger | Action Decomposition | Action Elimination | Hierarchical 
 \textbf{HD-$\states$}  &  % Brief summary of the approach
 \textbf{HD-$\actions$}  &  % MDPs, POMDPs, Slate-MDPs, Dec-POMDPs, etc
 \textbf{Adv.} &  % MDPs, POMDPs, Slate-MDPs, Dec-POMDPs, etc
 \textbf{Code} \\  % MDPs, POMDPs, Slate-MDPs, Dec-POMDPs, etc
\hline
\multicolumn{6}{|c|}{\textbf{Text Based Games}} \\
\hline
Zork~\cite{zahavy2018learn} & Zork is a \emph{text-based game} where the agent must interact via a text-based interface, having to choose from over a thousand possible actions per state. & \checkmark & \checkmark & \xmark & \checkmark~\tablefootnote{\url{https://github.com/TomZahavy/CB_AE_DQN}} \\
\hline 
\hline
\end{tabular}}
\end{table}

\textbf{zork} is an interactive text based computer game, created by a member of the MIT Dynamic 
Modeling Group in the late 1970s~\cite{zahavy2018learn}.
Given that text-based interactions are required in order for a player/agent to progress,
Zork offers an environment with large state and action spaces, with the later also being
implemented by natural language.
A natural language parser processes the text provided by the player, which following 
the sophisticated parsing process is turned into an action and execute.  
The game confronts the player with range of challenging puzzles and navigation tasks, 
requiring intricate action sequences to solve.
To solve this game an agent must be capable of both long-term planning, and dealing 
with random events, \eg attacks~\cite{zahavy2018learn}.  
Suitable network architectures are required for this game that can handle NLP tasks~\cite{zahavy2018learn}. 

\subsubsection{Card Games}

\begin{table}[h]
\resizebox{\columnwidth}{!}{
\begin{tabular}{ |p{3cm}||p{6cm}|p{1.5cm}|p{1.5cm}|p{1cm}|p{1cm}|}
 \hline
 \multicolumn{6}{|c|}{\textbf{Environments Overview}} \\
 \hline
 \textbf{Name} & % Name of the aglo
 \textbf{Description} &  % Wolpertinger | Action Decomposition | Action Elimination | Hierarchical 
 \textbf{HD-$\states$}  &  % Brief summary of the approach
 \textbf{HD-$\actions$}  &  % MDPs, POMDPs, Slate-MDPs, Dec-POMDPs, etc
 \textbf{Adv.} &  % MDPs, POMDPs, Slate-MDPs, Dec-POMDPs, etc
 \textbf{Code} \\  % MDPs, POMDPs, Slate-MDPs, Dec-POMDPs, etc
\hline
\hline
\multicolumn{6}{|c|}{\textbf{Card Games}} \\
\hline
DouDizhu~\cite{pmlr-v139-zha21a} & Three-player card game where two players have to team up against a landlord. The game features a large action space with 27,472 possible combinations. &  \xmark & \checkmark & \checkmark & \checkmark~\tablefootnote{\url{https://github.com/kwai/DouZero}~\tablefootnote{\url{https://github.com/kwai/DouZero}}} \\
\hline
\hline
\end{tabular}}
\end{table}

\textbf{DouDizhu} is a three-player shedding-type card game, where the objective is
for each player to empty their hand before the other players~\cite{pmlr-v139-zha21a}.
In this game two players (termed Peasants) must team up against a Landlord. 
The Peasants win if either of them is the first to have no cards left before the landlord.  
This game is challenging due to i.) the two Peasants having to learn to coordinate,
and ii.) the 27,472 card combinations, representing the action space~\cite{pmlr-v139-zha21a}.
Different subsets of actions are legal depending on the current hand.
There is no easy way to abstract the action space, as playing an improper card can result
in an instant loss~\cite{pmlr-v139-zha21a}.  

\subsubsection{Networks}

\begin{table}[h]
\resizebox{\columnwidth}{!}{
\begin{tabular}{ |p{3cm}||p{6cm}|p{1.5cm}|p{1.5cm}|p{1cm}|p{1cm}|}
 \hline
 \multicolumn{6}{|c|}{\textbf{Environments Overview}} \\
 \hline
 \textbf{Name} & % Name of the aglo
 \textbf{Description} &  % Wolpertinger | Action Decomposition | Action Elimination | Hierarchical 
 \textbf{HD-$\states$}  &  % Brief summary of the approach
 \textbf{HD-$\actions$}  &  % MDPs, POMDPs, Slate-MDPs, Dec-POMDPs, etc
 \textbf{Adv.} &  % MDPs, POMDPs, Slate-MDPs, Dec-POMDPs, etc
 \textbf{Code} \\  % MDPs, POMDPs, Slate-MDPs, Dec-POMDPs, etc
\hline
\multicolumn{6}{|c|}{\textbf{Networks}} \\
\hline
Intelligent Communication Jamming~\cite{e24101441} & Communication jamming decision making domain where two communication parties can adjust physical layer parameters to avoid jamming in a non-cooperative scenario.  & \xmark & \checkmark & \checkmark & \xmark \\
\hline
Multicast Scheduling Problem~\cite{li2022multicast} & The multicast scheduling problem requires the broadcasting of multiple messages over multiple channels. The objective is to minimizes the energy consumption of the base station and the latency of serving asynchronous requests from the mobile users. & \xmark & \checkmark & \xmark & \xmark \\
\hline
\end{tabular}}
\end{table}

\textbf{The Multicast Scheduling Problem:} 
Multicasting is a technique for efficiently transmitting common message from a base station 
to multiple mobile users in parallel~\cite{li2022multicast}.
The multicast scheduling problem consists of sending multiple message through multiple channels,
while simultaneously reducing the energy consumption of the base station, and reducing the latency
with which mobile users receive the messages.
The challenge is made more challenging due to requires being asynchronous.
The problem is challenging due to a large action space that must satisfy time-varying constraints.  

\textbf{Intelligent Communication Jamming:} 
Xu et al.~\cite{e24101441} study an intelligent jamming decision electronic warfare scenario,
in which two communication agents must adjust physical layer parameters to avoid blocking by
a jammer.
The scenario is considered from the perspective of the jammer (although in principle RL
could also be applied to the sender and receiver agents).
The domain features a MultiDescrete action spaces as must adust communication 
parameters including, modulation $\{M_1, M_2, ..., M_n\}$, transmission power 
$\{P_1, P_2, ..., P_m\}$ and communication frequency points $\{C_1, C_2, ..., C_l\}$.
The scenario is depicted in~\autoref{fig:jaming}.
\begin{figure}
\centering
\includegraphics[width=\columnwidth]{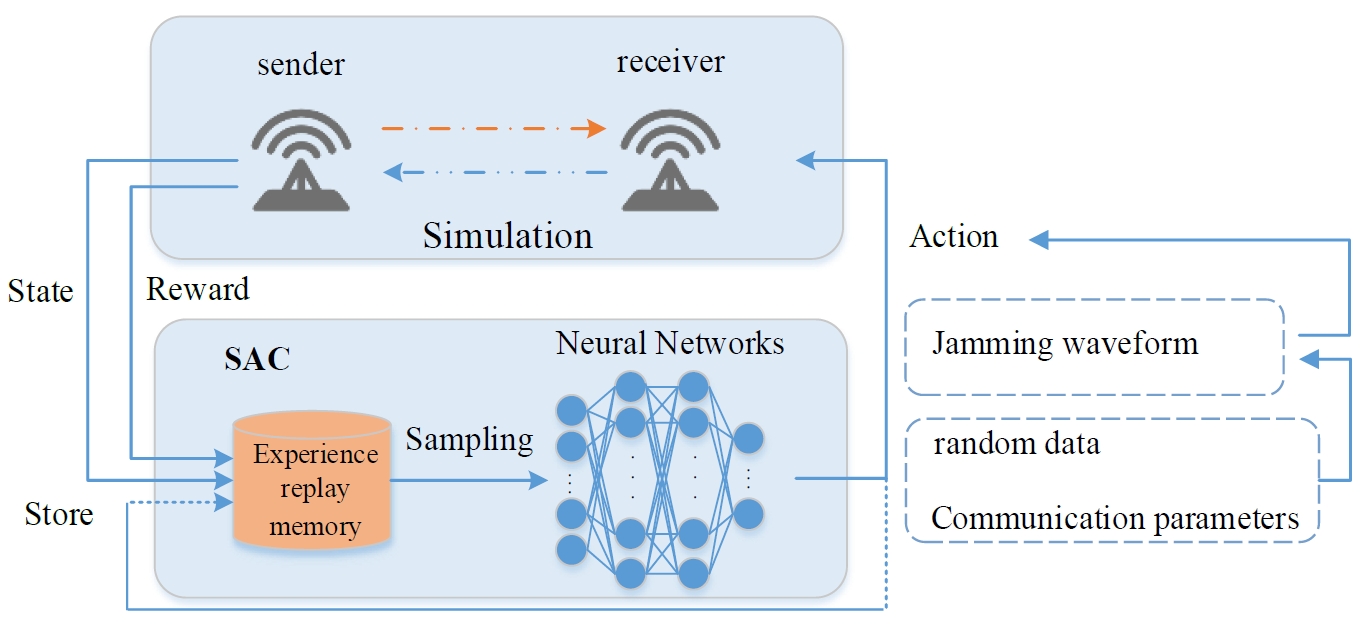}
\caption{Depiction of an intelligent communication jamming architecture (adopted from~\cite{e24101441}).}
\label{fig:jaming}
\end{figure}

\subsubsection{Recommender Environment} \label{sec:env:recommender_envs}

\begin{table}[h]
\resizebox{\columnwidth}{!}{
\begin{tabular}{ |p{3cm}||p{6cm}|p{1.5cm}|p{1.5cm}|p{1cm}|p{1cm}|}
 \hline
 \multicolumn{6}{|c|}{\textbf{Environments Overview}} \\
 \hline
 \textbf{Name} & % Name of the aglo
 \textbf{Description} &  % Wolpertinger | Action Decomposition | Action Elimination | Hierarchical 
 \textbf{HD-$\states$}  &  % Brief summary of the approach
 \textbf{HD-$\actions$}  &  % MDPs, POMDPs, Slate-MDPs, Dec-POMDPs, etc
 \textbf{Adv.} &  % MDPs, POMDPs, Slate-MDPs, Dec-POMDPs, etc
 \textbf{Code} \\  % MDPs, POMDPs, Slate-MDPs, Dec-POMDPs, etc
\hline
\multicolumn{6}{|c|}{\textbf{Recommender Environments}} \\
\hline
Recommender Environment~\cite{rohde2018recogym,2021RL4RS,pmlr-v97-chen19f,10.1145/3289600.3290999,ie2019reinforcement,afsar2022reinforcement} & Recommender systems where the agent is required to suggest a list (or a page) of options. See the section on Slate-MDPs for a formal definition of this problem~\autoref{sec:slateMDPs}. & \checkmark & \checkmark & \xmark & \checkmark~\tablefootnote{\url{https://github.com/fuxiAIlab/RL4RS}, \url{https://github.com/criteo-research/reco-gym}}\\
\hline
\hline
\end{tabular}}
\end{table}

While the Slate-MDP problem formulation could be relevant for a 
range of application areas -- \eg human-in-the-loop \aco environments -- 
the majority of works in this area are implemented for and
evaluated on recommendation systems
~\cite{pmlr-v97-chen19f,10.1145/3289600.3290999}.
The recommender system problem can essentially be formulated as follows:
given a huge corpus of content, can we find an efficient policy small
fractions of content that a user will be interested in~\cite{10.1145/3289600.3290999},
e.g., TV show recommendations on Netflix and Amazon.
Taking into account user preferences here is the key, as recommender 
systems are tasked with recommending the right item, to the
right user, at the right time.
Again, relating to \aco, given a group of specialised administrators,
 a recommender system could be tasked with flagging up activities 
that it deems suspicious to the admin who is most interested (and
most likely to resolve identify and solve the matter).
A key component of the recommender system training process
is that the user provides feedback through an action from 
the slate being selected and executed, \ie the movie is played
for a certain duration.
Based on this feedback the system can adjust its model and make
further recommendations.
Put simply, at each time step, the system displays $k$ items
(presenting a slate of $k$ actions), the user then picks an action,
feedback is provided, the system moves on to the next state, and
a new slate based is made~\cite{pmlr-v97-chen19f}. 
In industrial settings recommender systems are confronted 
with large state and action spaces, due to the large number 
of items from which to select recommendations.
To complicate the matter the set of items from which the agent
can choose a slate is often non-stationary,
and often growing, leading to an ever larger action space~\cite{10.1145/3289600.3290999}.
User preferences are also non-stationary thereby introducing 
drift~\cite{10.1145/3289600.3290999}.
The observation space is large, as it can feature both static
features, \eg demographic, declared interests, and other attributes, as well
as context (time of the day, user location), and encodings of past behaviour.
Efficient methods are therefore required for encoding a user's history.
The scenario is depicted in \autoref{fig:recomendation_system}.
\begin{figure}
\centering
\includegraphics[width=\columnwidth]{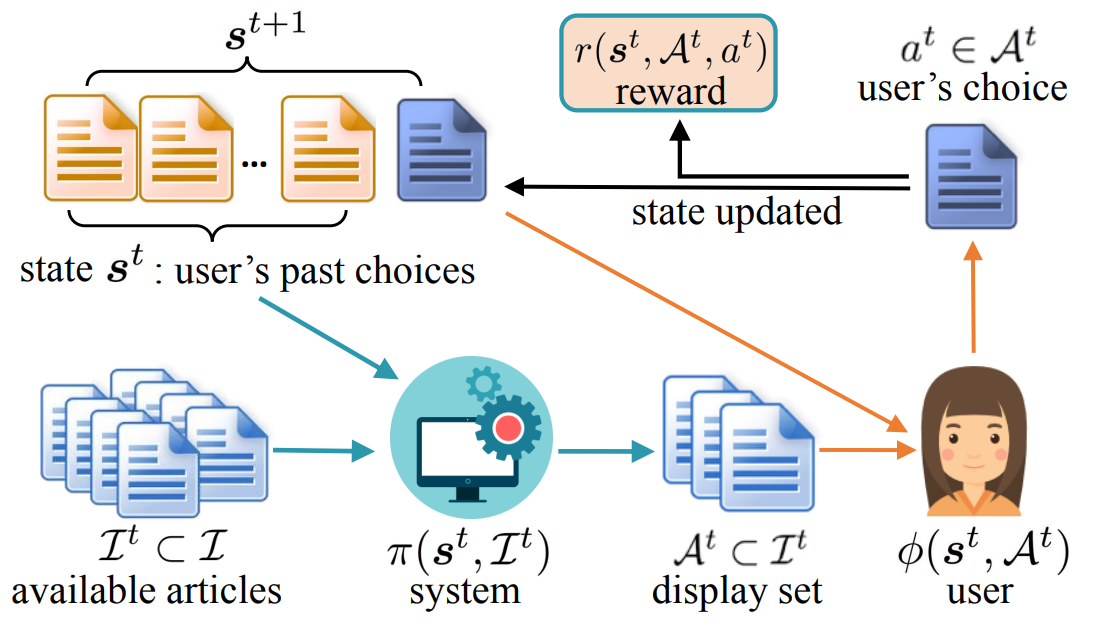}
\caption{Depiction of a recommendation system (adopted from~\cite{pmlr-v97-chen19f}).}
\label{fig:recomendation_system}
\end{figure}

\subsubsection{Fully Cooperative Multi-Agent Environments}

\begin{table}[h]
\resizebox{\columnwidth}{!}{
\begin{tabular}{ |p{3cm}||p{6cm}|p{1.5cm}|p{1.5cm}|p{1cm}|p{1cm}|}
 \hline
 \multicolumn{6}{|c|}{\textbf{Environments Overview}} \\
 \hline
 \textbf{Name} & % Name of the aglo
 \textbf{Description} &  % Wolpertinger | Action Decomposition | Action Elimination | Hierarchical 
 \textbf{HD-$\states$}  &  % Brief summary of the approach
 \textbf{HD-$\actions$}  &  % MDPs, POMDPs, Slate-MDPs, Dec-POMDPs, etc
 \textbf{Adv.} &  % MDPs, POMDPs, Slate-MDPs, Dec-POMDPs, etc
 \textbf{Code} \\  % MDPs, POMDPs, Slate-MDPs, Dec-POMDPs, etc
\hline
\multicolumn{6}{|c|}{\textbf{Fully Cooperative Multi-Agent Environments}} \\
\hline
PettingZoo~\cite{terry2021pettingzoo} & Library featuring numerous domains that could be viewed through the lense of applying a single agent joint-action learning approach to domains with a MultiDescrete action space. & \checkmark & \checkmark & \xmark & \checkmark\tablefootnote{\url{https://pettingzoo.farama.org/}} \\
\hline
SMAC~\cite{samvelyan2019starcraft,samvelyan19smac} & Benchmarking environment based on the popular real-time strategy game StarCarft II. & \boldcheckmark & \boldcheckmark & \boldcheckmark & \boldcheckmark\tablefootnote{\url{https://github.com/oxwhirl/smac}} \\
\hline
Traffic Simulations~\cite{lopez2018microscopic} & Microscopic Traffic simulation tool for traffic research. Allows for the implementation of complex distributed traffic light control scenarios. & \checkmark & \checkmark & \xmark & \checkmark~\tablefootnote{\url{https://www.eclipse.org/sumo/}} \\
\hline
Iroko~\cite{ruffy2018iroko} & Flexible, configurable emulator for benchmarking data-driven congestion control on networks. & \checkmark & \checkmark & \checkmark & \checkmark\tablefootnote{\url{https://github.com/dcgym/iroko}} \\
\hline
Team-Games~\cite{JMLR:v17:15-417,bloembergen2010lenient,wei2018multiagent,bloembergen2010lenient,palmer2018negative,palmer2018lenient,palmer2020independent}
&
Various team games from the multi-agent reinforcement learning literature designed to evaluate the extent to which approaches are susceptible toward multi-agent learning pathologies. Includes both stateless game, and games with high-dimensional states/observations. 
& \checkmark & \checkmark & \xmark & \checkmark \\
\hline
Half Field Offense~\cite{HFO}
&
Half Field Offense is a soccess simulation where players are either designated as attackers or defenders.
& \checkmark & \checkmark & \checkmark & \checkmark~\tablefootnote{\url{https://github.com/LARG/HFO}} \\
\hline
\end{tabular}}
\end{table}

Many of the MultiDescrete problem scenarios discussed in this 
report can infact the viewed as cooperative learning scenarios,
\eg  
the discretised continuous control domains discussed in \autoref{Sec:DCCD}.
Within this scenario each actuator can be viewed as an agent.
As we shall see in \autoref{sec:action_decomposition} approaches in this
area are prone to some of the challenges encountered in multi-agent learning.
Indeed, the multi-agent learning literature considers single 
agents solutions applied the above problem formulation as joint-actions 
learners, where one agent learns a policy for all agents in the system,
while the alternative is concurrent learning, where agent's learn 
a policy independently~\cite{palmer2020independent}. 
Indeed, one of the motivating factors for turning to multi-agent learning
is the notion that, while single agent learning approaches perform well
when applied to joint-action learning problems, the approaches often
do not scale well, as increasing the number of agents results in an 
exponential increase in the size of the observation-action space
~\cite{hernandez2017survey,matignon2007hysteretic,rashid2018qmix,
son2019qtran,sunehag2017value,guptacooperative,
castellini2019representational,devlin2011theoretical}. 
Indeed, in action space that allows each of $N$ actoins to 
take an action from a set $\actions_{agent}$ we have an 
exponentially large action space of size $\rvert\\actions_{agent}\rvert^N$.
Therefore, the multi-agent learning literature provides a 
numerous environments capable of confronting agents with 
high dimensional observation spaces and high dimensional 
action spaces capable of stress testing approaches designed 
to address these issues. 
Below we provide an overview of suitable domains and gym frameworks. 

\textbf{PettingZoo Library:} Terry et al.~\cite{terry2021pettingzoo} introduced 
the PettingZoo library along with an accompanying agent environment cycle games
model, providing a diverse set of multi-agent learning environments with a 
Python API to accelerate multi-agent reinforcement learning research.
The motivation for implementing it was to provide a multi-agent reinforcement 
learning equivalent of the OpenAI Gym that is frequently used for single agent
reinforcement learning~\cite{brockman2016openai}. 
The library provides a range of domains that can be viewed through the lens
of MultiDiscrete action learning, \eg the cooperative multi-agent control 
domains provided by the Stanford Intelligent Systems Laboratory (SISL) would provide
suitable benchmarking domains for approaches aimed at tackling discretized 
control environments, confronting learners with both a high-dimensional
combinatorial action space and, through the multiple observation points,
a high dimensional observation space
~\footnote{\url{https://pettingzoo.farama.org/environments/sisl/}} (See~\autoref{fig:SISL} 
for a depiction of the relevant domains). 
\begin{figure}[h]
\centering     %%% not \center
\subfloat[Mult-Agent Walker]{\label{fig:envs:MAWalker}\includegraphics[height=35mm]{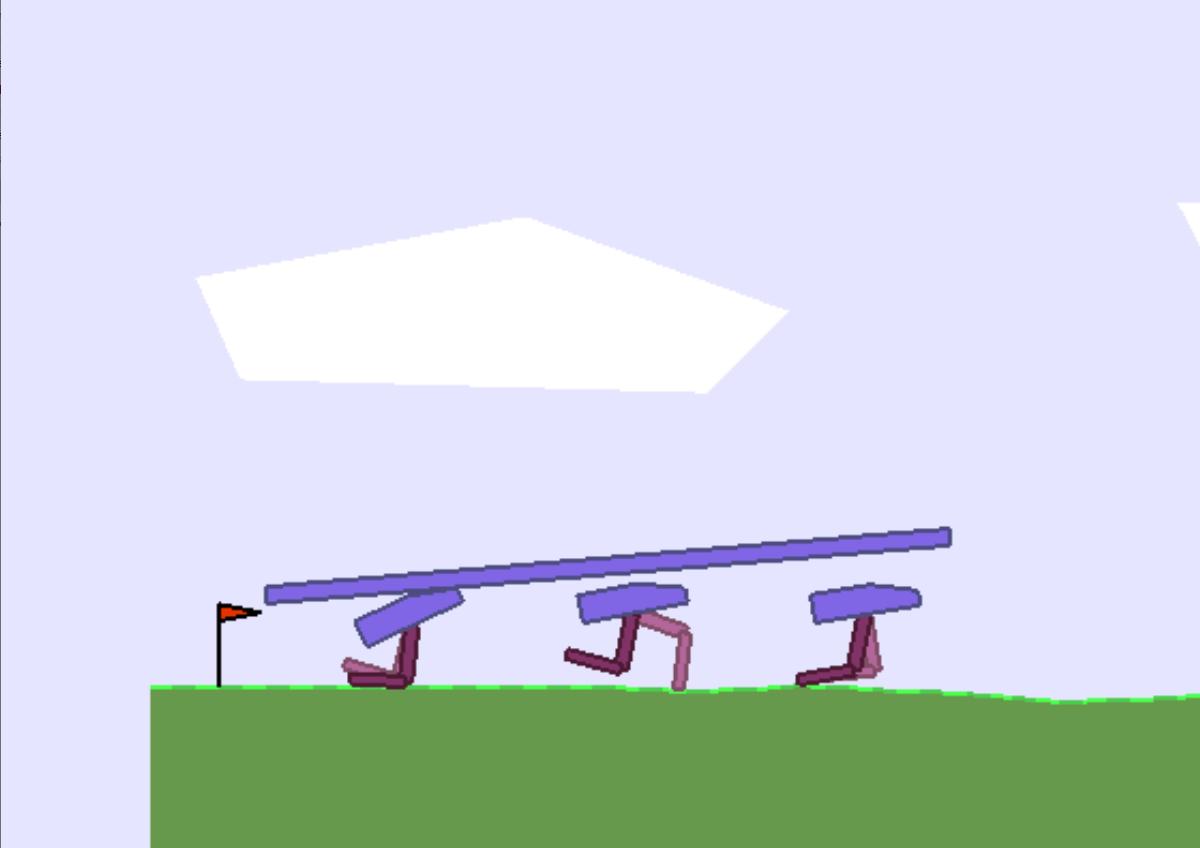}}
\hspace{5mm}
\subfloat[Pursuit]{\label{fig:envs:Pursuit}\includegraphics[height=35mm]{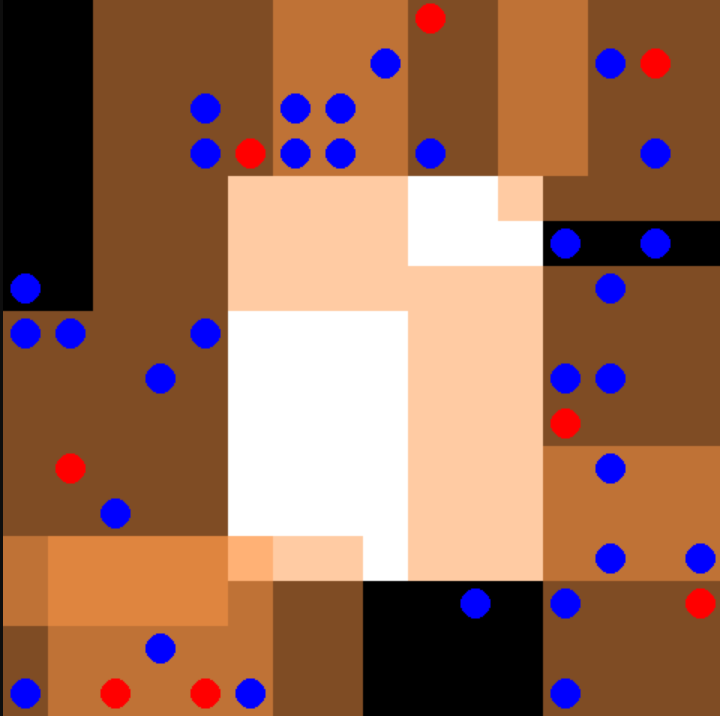}}
\hspace{5mm}
\subfloat[Waterworld]{\label{fig:envs:Waterworld}\includegraphics[height=35mm]{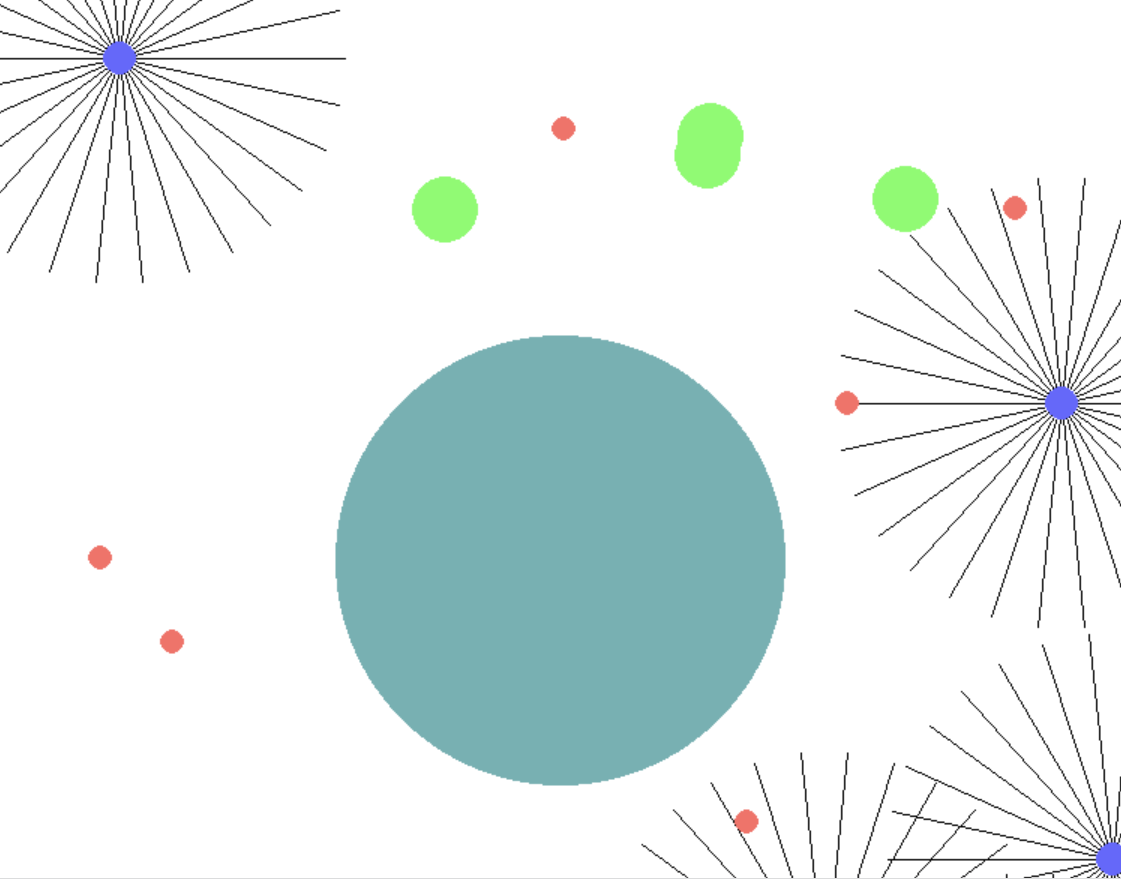}}
\caption{Cooperative multi-agent control benchmark environments introduced by Stanford Intelligent Systems Laboratory (SISL) that would make 
interesting benchmarking domain for discretized control approaches.}
%\label{fig:SISL}
\end{figure}

\textbf{StarCraft Multi-Agent Challenge (SMAC):}
SMAC is a partially-observable benchmarking environment based 
on the popular real-time strategy game 
StarCarft II~\cite{samvelyan2019starcraft,samvelyan19smac}.
It confronts learners with a micromanagement task, where combat units
are typically controlled by an independent agent that much act based 
on local observations.
However, the environment also presents an opportunity for benchmarking
joint-action learners, given that it features many of the properties
that we listed as desirable in \autoref{sec:target_env_properties}, 
including high dimensional action and observation spaces, as well
as the facility for adversarial learning. 
It is worth noting that this domain has already been used by 
Farquhar et al.~\cite{pmlr-v119-farquhar20a} for evaluating
a curriculum leanring approach for growing action spaces. 
\begin{figure}
\centering
\includegraphics[width=\columnwidth]{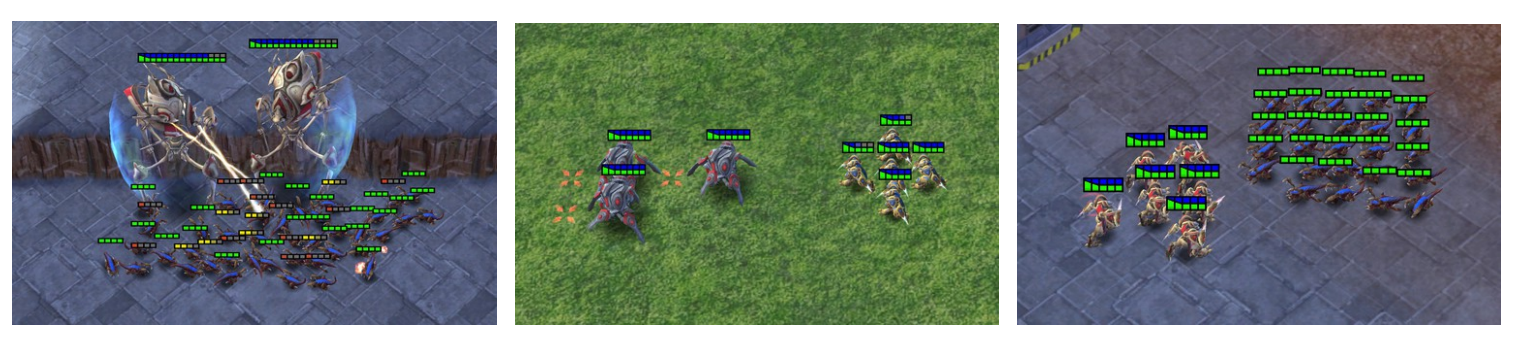}
\caption{Screenshots from three SMAC scenarios (adopted from~\cite{samvelyan2019starcraft}).}
\label{fig:SMAC}
\end{figure}

\textbf{Microscopic Traffic Simulation:}
Microscopic traffic simulations~\cite{lopez2018microscopic} provide a
valuable tool for research on traffic scenarios, as well as benchmarking
domains the features that match the majority of our requirements, perhaps
with the exception of an adversarial component -- although addressable 
through robust adversarial reinforcement learning, \eg an adversary
capable of \say{sabotaging} a traffic light in a grid. 
Interesting scenarios that have been explored in the multi-agent 
reinforcement learning literature include distributed 
traffic light control\cite{pmlr-v139-zimmer21a}, and the use
of multi-agent reinforcement learning to simulate agents with
different levels of aggression~\cite{bacchiani2019microscopic}.

\textbf{Distributed Data Center Control:}
Explores the question of whether data-driven congestion control
agents using deep reinforcement learning can learn optimal
network policies.
The Iroko emulator allows the benchmarking of approaches in this
setting~\cite{ruffy2018iroko}.
Iroko is flexible, allowing the modelling of different network
topologies, congestion and deployment scenarios. 
It provides an OpenAI gym interface, and therefore has become
a popular tool for multi-agent reinforcement learning benchmarking~\cite{pmlr-v139-zimmer21a}.

\textbf{Team-Games}
As we shall see under approaches for high dimensional action spaces in \autoref{sec:hdas_approaches}, 
one category of methods uses what can be viewed as a multi-agent approach towards composing
a combinatorial action.
Authors in this area of the literature have noted that their methodologies can fail to 
learn cooperate and converge upon a reasonable policy when implemented with independent
learning approaches, and as a result turn towards advanced multi-agent reinforcment learning
approaches (\eg QMix~\cite{rashid2018qmix}) to facilitate cooperation.
However, this raises the question of the extent to which the resulting implementations are
indeed robust to the multi-agent learning pathologies discussed in \autoref{sec:marl_concepts},
in particular at scale, \ie when the action is the result of a decomposition into a large 
number of agents.
Here the multi-agent reinforcement learning literature offers a range of games designed 
to tease out how suceptable an approach is towards a particular sub-set of pathologies.
A large number of these games are even stateless, therefore offering focused benchmarking
domains to try out novel approaches for testing the action composition processes
~\cite{JMLR:v17:15-417,bloembergen2010lenient,wei2018multiagent,bloembergen2010lenient}. 
Meanwhile, in other work, the same problem formulation has been transolated into 
DecPOMDPs with a compareable reward space~\cite{palmer2018negative}.
